# Supplementary material for: Towards a Generative Approach for Emotion Detection and Reasoning
Source: arXiv:2408.04906 source file (2024-08-09)
Supplement: Supplementary file 1 [file appendix.tex]

\section{Appendix: Context Generation Prompts}
\label{appendix_a}
Table \ref{tab:isear_context} and \ref{tab:tec_context} show the prompts used for context generation. The instruction and type of context are chosen according to the dataset creation process and domain.

\begin{table*}[h]
    \centering
    \begin{tabular}{p{0.9\linewidth}}
    \hline
    Generate the context for the situation described in the input.\\
Here are some examples: \\ \\

Input: I did not do the homework that the teacher had asked us to do. I was scolded immediately.\\
Context: This situation suggests that the person is a student who did not complete their homework as instructed by their teacher. \\ \\

Input: My parents were out and I was the eldest at home.  At midnight a male stranger phoned us and spoke to me in a rough language. I hung up and heard someone walking outside our door. \\
Context: This situation describes a home invasion or a potential break-in which could have been very frightening for the person at home, and may have left them feeling vulnerable and afraid.\\ \\

Input: I received a letter from a distant friend.\\
Context: The input suggests that the author has received a letter from a friend who is far away. \\ \\

Input: On days when I feel close to my partner and other friends. When I feel at peace with myself and also experience a close contact with people whom I regard greatly. \\
Context: The input describes the author's feelings on certain days when they feel a strong emotional connection with their partner and close friends. \\ \\

Input: Every time I imagine that someone I love or I could contact a serious illness, even death. \\
Context: The input suggests that the author experiences anxiety or fear at the thought of a loved one or themselves falling ill or dying. \\ \\

Input: \{input text\}\\
Context:\\
        \hline
    \end{tabular}
    \vspace{-0.1in}
    \caption{Prompt for context generation for ISEAR dataset.}
    \label{tab:isear_context}
    \vspace{-0.1in}
\end{table*}

\begin{table*}[h]
    \centering
    \begin{tabular}{p{0.9\linewidth}}
    \hline
    Generate the context for the tweet in the input. \\
Here are some examples: \\ \\

Input: the moment when you get another follower and you cheer. \\
Context: The tweet expresses personal excitement at gaining a new follower on a social media platform. \\ \\

Input: sounds awful but a lot of people are dying recently :((  \\
Context: The tweet expresses personal concern about recent reports of multiple deaths.\\ \\

Input: Don't believe the lies, look me in the eyes- please don't be scared of me\\
Context: The tweet expresses a plea for someone not to be afraid and to trust the speaker. \\ \\

Input: been awake since 4:30am. too tired for black friday fun. \\
Context: The tweet appears to be a personal message from an individual who has been awake since 4:30am, expressing exhaustion and lack of interest in participating in Black Friday shopping activities.  \\ \\

Input: Father forgive me for my and help me live boldly in Your \#truth \#GloryOfTheCross\\
Context: The tweet appears to be a personal message from an individual seeking forgiveness from God and expressing a desire to live boldly in accordance with Christian values. \\ \\

Input: \{input text\}\\
Context:\\
        \hline
    \end{tabular}
    \vspace{-0.1in}
    \caption{Prompt for context generation for \#Emo dataset.}
    \label{tab:tec_context}
    \vspace{-0.1in}
\end{table*}
